# Supplementary material for: Mirror-Aware Neural Humans
Source: arXiv:2309.04750 source file (2024-05-15)
Supplement: Supplementary file 1 [file supp_novel_views.tex]

\begin{figure}[!ht]
\centering
\includegraphics[width=1.0\linewidth,trim={0.0cm 0.0 0.0cm 0.0cm},clip]{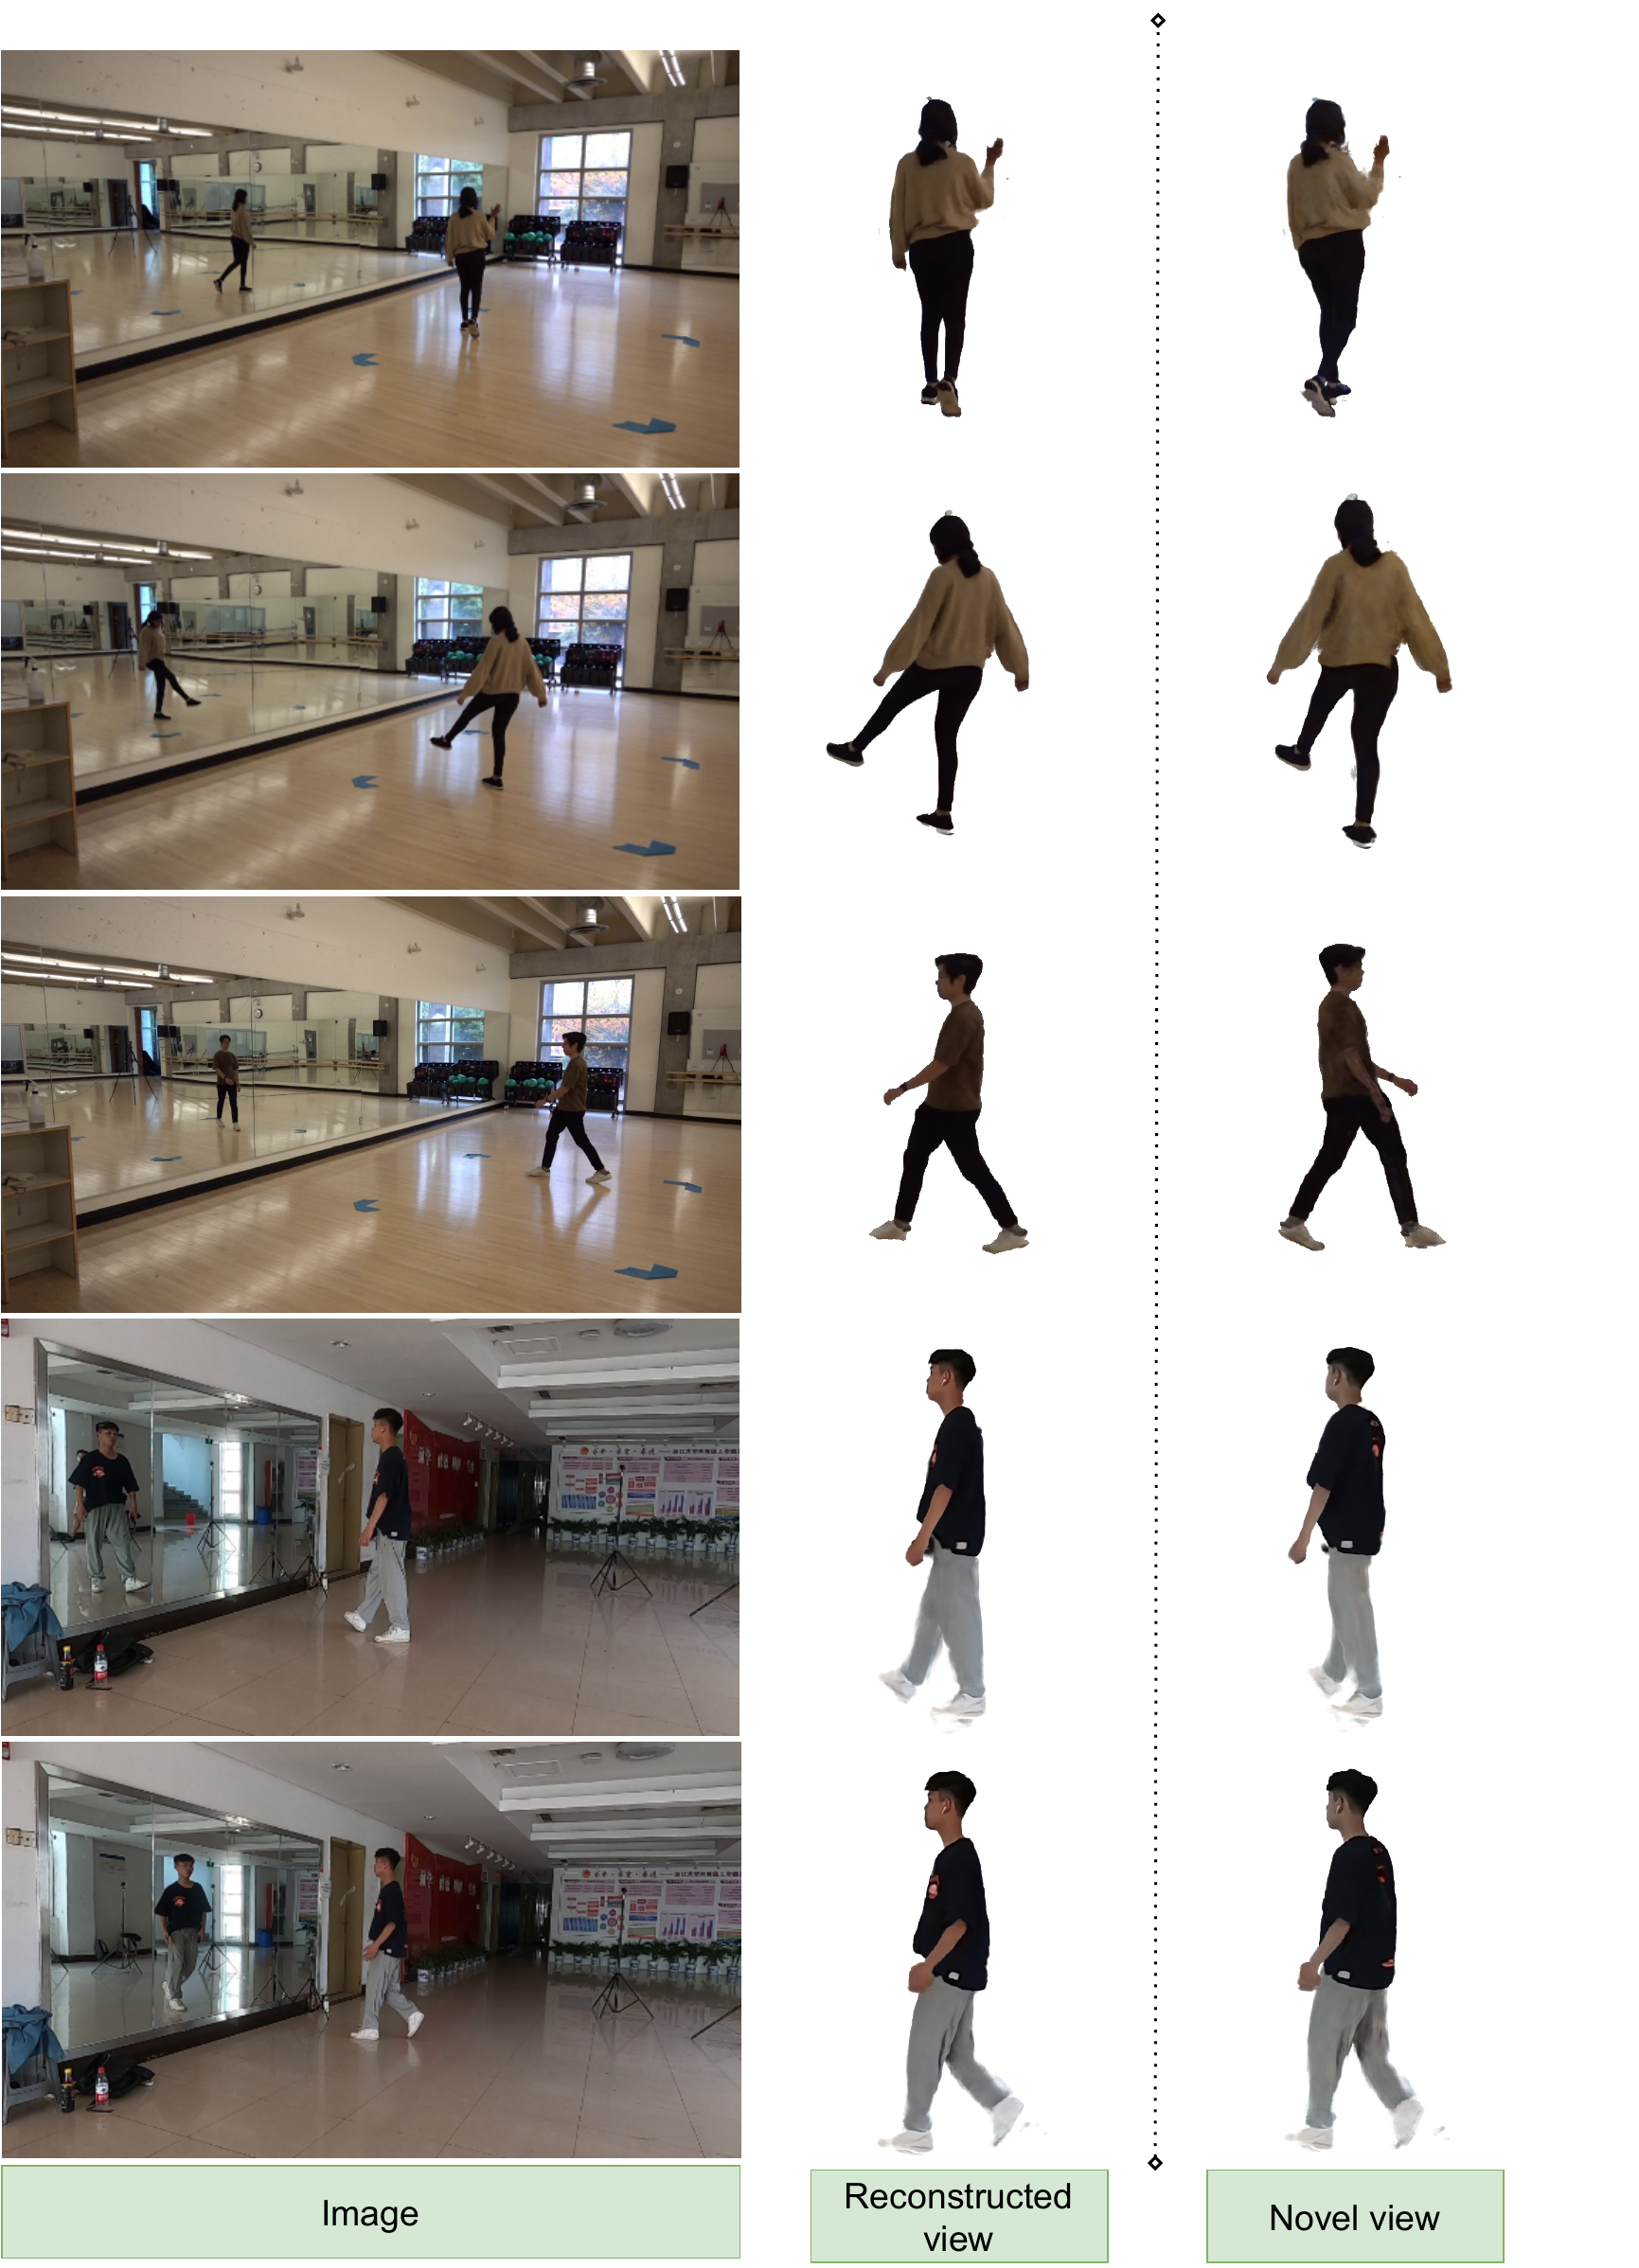}
  \caption{\textbf{Novel view synthesis results}. The learned reconstruction is a proper 3D model that can be rotated to novel views.}
\label{fig:supp_novel_views} 
\end{figure}
