# Supplementary material for: Mirror-Aware Neural Humans
Source: arXiv:2309.04750 source file (2024-05-15)
Supplement: Supplementary file 2 [file supp.tex]

% % CVPR 2024 Paper Template; see https://github.com/cvpr-org/author-kit

% \documentclass[10pt,twocolumn,letterpaper]{article}

% %%%%%%%%% PAPER TYPE  - PLEASE UPDATE FOR FINAL VERSION
% \usepackage{cvpr}              % To produce the CAMERA-READY version
% % \usepackage[review]{cvpr}      % To produce the REVIEW version
% % \usepackage[pagenumbers]{cvpr} % To force page numbers, e.g. for an arXiv version
% \input{packages}

% % Import additional packages in the preamble file, before hyperref
% \input{preamble}

% % It is strongly recommended to use hyperref, especially for the review version.
% % hyperref with option pagebackref eases the reviewers' job.
% % Please disable hyperref *only* if you encounter grave issues, 
% % e.g. with the file validation for the camera-ready version.
% %
% % If you comment hyperref and then uncomment it, you should delete *.aux before re-running LaTeX.
% % (Or just hit 'q' on the first LaTeX run, let it finish, and you should be clear).
% \definecolor{cvprblue}{rgb}{0.21,0.49,0.74}
% \usepackage[pagebackref,breaklinks,colorlinks,citecolor=cvprblue]{hyperref}
% \usepackage{nopageno} % remove page nos

% %%%%%%%%% PAPER ID  - PLEASE UPDATE
% \def\paperID{12} % *** Enter the Paper ID here
% \def\confName{3DV\xspace}
% \def\confYear{2024\xspace}

% %%%%%%%%% TITLE - PLEASE UPDATE
% \title{Supplemental Material for Mirror-Aware Neural Humans}


% %%%%%%%%% AUTHORS - PLEASE UPDATE

% % \author {Daniel Ajisafe$^1$ \qquad James Tang$^1$ \qquad Shih-Yang Su$^1$ \qquad Helge Rhodin$^1$ \qquad Bastian Wandt$^2$ \\
% % {\tt\small (dajisafe,shihyang,rhodin)@cs.ubc.ca, tangytob@student.ubc.ca, bastian.wandt@liu.se} \\
% % The University of British Columbia$^1$ \\
% % Linköping University$^2$
% % }

% % \and
% % James Tang\\
% % {\tt\small tangytob@student.ubc.ca} \\
% % \and
% % Shih-Yang Su\\
% % {\tt\small shihyang@cs.ubc.ca} \\
% % \and
% % Helge Rhodin\\
% % {\tt\small rhodin@cs.ubc.ca}\\
% % The University of British Columbia\\
% % Institution1 address\\
% % For a paper whose authors are all at the same institution,
% % omit the following lines up until the closing ``}''.
% % Additional authors and addresses can be added with ``\and'',
% % just like the second author.
% % To save space, use either the email address or home page, not both
% % \and
% % Bastian Wandt\\
% % Linköping University\\
% % First line of institution2 address\\
% % {\tt\small bastian.wandt@liu.se}
% % }

% % \author{Daniel Ajisafe \\
% % {\tt\small dajisafe@cs.ubc.ca}
% % \and
% % James Tang\\
% % {\tt\small tangytob@student.ubc.ca} \\
% % \and
% % Shih-Yang Su\\
% % {\tt\small shihyang@cs.ubc.ca} \\
% % \and
% % Helge Rhodin\\
% % {\tt\small rhodin@cs.ubc.ca}\\
% % % The University of British Columbia\\
% % % Institution1 address\\
% % % For a paper whose authors are all at the same institution,
% % % omit the following lines up until the closing ``}''.
% % % Additional authors and addresses can be added with ``\and'',
% % % just like the second author.
% % % To save space, use either the email address or home page, not both
% % \and
% % Bastian Wandt\\
% % Linköping University\\
% % % First line of institution2 address\\
% % {\tt\small bastian.wandt@liu.se}
% % }

% \begin{document}
% \maketitle


% In addition to the results in the main paper, we provide more qualitative results and implementation details. The supplemental video shows the results in motion.

% \input{figures/step2_recon.tex}



% \section{Additional qualitative 3D Reconstruction Results}
% Figure~\ref{fig:virtual_pose}  demonstrates the capability of Mirror-Aware Neural Humans (Step 2 output) to reconstruct challenging poses where existing 3D pose estimators are prone to fail. The lying down pose is representative both for strong self occlusions, which necessitates the second mirror view or other means of multi-view recording, and for \danred{extreme vertical poses}, which goes against the bias towards standing poses learning-based approaches have.

% \section{Novel View and Pose Synthesis}

% \input{figures/supp_novel_views.tex}
% Figure~\ref{fig:supp_novel_views} shows novel view synthesis results that reveal an accurate 3D reconstruction of the monocular input images. Notably, the model-free nature enables reconstructing unique shapes such as long hair and loose clothing (first two rows), body accessories such as wristwatch (central row), and texture details such as logos (last two rows).

% % reconstructing unique shapes such as the beard (first two rows), loose clothing (central two rows), and texture details such as logos (last two rows).

% \input{figures/mirror_retarget.tex}
% \input{figures/skel_3D_reprojection}

% Figure~\ref{fig:mirror_retarget} simulate one of the learned volumetric body models in an unseen mirror arrangement, requiring both novel view (mirror) and novel pose \da{from a different actor.}

% % (transferred from source). %The latter, Figure~\ref{fig:mirror_retarget} is more challenging as it is difficult to reconstruct such a simulation without learning the mirror geometry properly. 
% This highlights the effectiveness of our automatic mirror normal estimation (discussed in the main paper).
% % \input{figures/before_after_refine.tex}
% % \section{Benefit of the Volumetric Pose Refinement}
% % Figure~\ref{fig:before and after} shows our 3D skeleton pose reconstruction before and after the refinement with the volumetric body model (Step 3). The 3D pose overlay on the input image shows that the joint refinement of pose and shape through mirror constraints improves significantly, particularly on extreme poses.




% %# 1 failure case "add"

% \section{Effect of Regularization Constraints}


% Figure~\ref{fig:ablation-location} Left measures the importance of the smoothness term on our 3D reconstruction objective and shows its robustness to different weights. The smoothness term on orientation with a weight of 1.0 minimizes the 3D reconstruction error (measured in P-MPJPE). Figure~\ref{fig:ablation-location} Right carries out the same ablation on the body joint location smoothness term, with a scale of 0.22, leading to the best results on the validation sequence.

% \input{figures/loc_smooth_scale.tex}


% \comment{
% \section{Camera and ground plane initialization}

% To make the 3D reconstruction from a mirror scene practical, we \danteal{solve for} the orientation and position of the mirror and camera
% by utilizing that 
% the person is, at least in some frames, upright and moves on a flat orthogonal ground plane,
% such that the 3D neck position $\vp_\text{neck}$ is a function of height $h$ and ground normal $\vn_g \in\Real^3$,
% \begin{equation}
%     \vp_\text{neck} = (\vp_\text{ankle} + \vn_g h)
%     \label{eq:head}.
% \end{equation}
% We select poses $\vq^{(t)}$ 
% \danteal{from detections} where the person is standing up-right by measuring the angles from shoulder to the pelvis, pelvis to knee, and knee to ankle, and filter those where the sum of their deviation from $180^\circ$ exceeds $34^\circ$.
% %
% \danteal{By applying Eq.~\ref{eq:head}} on three or more detected poses in combination with the perspective projection from 3D coordinates $\vp$,
%     \begin{equation}
%     \vq = \mK \vp,
%     \text{ where }
% \mK = 
% \begin{pmatrix}
% f & 0 & o_1 & 0\\
% 0 & f & o_2 & 0\\
% 0 & 0 & 1 & 0
% \end{pmatrix},
% \label{eq:projection}
% \end{equation}
% %
% with $(o_1,o_2)$ the image center,
% suffices to reconstruct the desired ground plane normal $\vn_g\in \mathbb{R}^3$ and focal length $f$ using RANSAC~\cite{fischler1981random}. 
% % Such approach was described in \cite{fei2021single} but no source code is available.
% }

% \section{Mirror Matrix Derivation}

% We provide further details on the mirror matrix derivation. Following~\cite{rotation_arbitrary, schwertz2012field}, we define a mirror operation $\mA$ that mirrors points across the mirror plane $\pi$. This operation includes a rotation and reflection, and can be described using the plane equation,

% \begin{gather}
%     n_{x}x + n_{y}y + n_{z}z + d = 0 %, \text{ with,}
% \label{eq:mirror_plane}
% \end{gather}
% % and, $d$ can be re-written as, 
% %
% where $d = -\vm \cdot \vn_{m}$ is the distance of the mirror plane to the camera origin. Generally, $\vm$ can be any point on the plane that defines the plane's location, and in this case, the mirror location is chosen as the point between the real and mirrored person. $\vn_{m}$ is the normal of the mirror that defines the orientation of the plane. Hence, we can derive the virtual camera through a mirror matrix $\mA$ that reflects point through the plane in Eq.~\ref{eq:mirror_plane} using $\mA = \mI - 2 \vn_m\vn_m^T$~\cite{householder1958unitary} where $\mI$ is a $3\times3$ identity matrix. The mirror matrix $\mA$  can be expanded as,
% %
% \begin{equation}
% \mA =
% \begin{bmatrix}
% 1 & 0 & 0 \\
% 0 & 1 & 0 \\
% 0 & 0 & 1 \\
% \end{bmatrix}
% -
% 2 \cdot 
% \begin{bmatrix}
% n_{x}\\n_{y}\\n_{z}
% \end{bmatrix}
% \cdot 
% \begin{bmatrix}
% n_{x} & n_{y} & n_{z}
% \end{bmatrix} \text{ or,}
% \end{equation}
% %
% \begin{equation}
% \mA =
% \begin{bmatrix}
% (1-2n_{x}^{2}) & -2n_{y}n_{x} & -2n_{z}n_{x} \\
% -2n_{y}n_{x} & (1-2n_{y}^{2}) & -2n_{y}n_{z} \\
% -2n_{z}n_{x} & -2n_{y}n_{z} & (1-2n_{z}^{2}) \\
% \end{bmatrix},
% \end{equation}
% %
% which can be fully expressed as a $4\times4$ affine transformation matrix such that,
% %
% \begin{equation}
% \mA =
% \begin{bmatrix}
% (1-2n_{x}^{2}) & -2n_{y}n_{x} & -2n_{z}n_{x} & -2n_{x}d\\
% -2n_{y}n_{x} & (1-2n_{y}^{2}) & -2n_{y}n_{z} & -2n_{y}d\\
% -2n_{z}n_{x} & -2n_{y}n_{z} & (1-2n_{z}^{2}) & -2n_{z}d\\
% 0 & 0 & 0 & 1
% \end{bmatrix},
% \end{equation}
% with $\vn_m = [n_x,n_y,n_z]$ the mirror normal and $d$ is the distance between the camera and mirror (both quantities are from Step~1 in the main document.
% %with $d$ the mirror distance as before.
% %Since this mirror matrix maps points from one side of the mirror to the other, and the real camera is at the origin, this mirror matrix 
% By defining the real camera to be at the origin pointing along the z-axis, $\mA$ maps points from the real to the virtual camera using the following, 
% \begin{equation}
% \begin{bmatrix}
% \bar{x}\\\bar{y}\\\bar{z}
% \end{bmatrix} = 
% \mA 
% \cdot 
% \begin{bmatrix}
% x\\ y\\ z
% \end{bmatrix}
% \end{equation}
% %


% % The orientation of the virtual camera is hence $\bar{\mR} = \mA_{3\times3}^{\top}$, the inverse of the top-left part of $\mA$, and camera position $\bar{c} = -2\vn_m d$ is the negative of the last column of $\mA$.
% % Note that $\bar{\mR}$ is from the orthogonal group $O(3)$ %but not from $SO(3)$ 
% % as it includes a reflection component given by the mirror. Also 
% Note that the orientation of the virtual camera switches to a left-hand coordinate system (LH)~\cite{Rodrigues, schwertz2012field} based on the reflection component in $\bar{\mR}$.
% %, as shown in Figure \danred{2} in the main paper.

% %\input{figures/segment.tex}

% \input{tables/bbox_iou_ratio}

% \section{Separating Real and Mirror Poses}

% % Unlike [14], we do not use manually annotated 2D pose but use the Alphapose [13] detector, which outputs a set of 2D poses for every frame. 
% Since human pose detectors are not completely accurate, we drop frames where the pose prediction is below half of the height of a valid pose visually. On the MirrorHuman-eval dataset, we use the available GT focal length and remove detections on bystanders and correct ambiguous real-to-mirror associations using the distance to the 2D GT annotation. Note that this ensures that we work with automatic detections as available in practice, containing slight inaccuracies, while leaving complete mis-detections or assignments out of the equation to aid a fair comparison to previous methods using 
% %\textcolor{red}{
% manually annotated ground truth 2D annotations. Note that this correction is only applied to the \emph{MirrorHuman-eval} dataset 
% %to be comparable 
% and only to very few frames and cameras; only for camera 2 (2 mismatches out of 1571 frames) and camera 5 (4 mismatches out of 1377 frames). 

% %2D detection bounding box 
% To analyze the effect of frames with occlusion compared to frames without, we measure the IOU between the bounding boxes for the virtual and real person. We select the one with a high confidence above 20\%  and quantify the amount of occluded frames in Table~\ref{tab:box_iou}. Only very few frames show occlusions but these are important to address.

% \section{Optimization and Training Details}

% In Step 1, we solve for the focal length and initial ground plane by solving a system of equations using Singular Value Decomposition (SVD) 
% %on a cluster CPU 
% for 20K RANSAC iterations. In Step 2, we jointly optimize for the joint rotations $\vtheta$, pelvis position $\vp_\text{pelvis}$, bone lengths  $\vell$, and joint rotations  $\vtheta$ (as explained in the main document)
% %to learn the underlying pose during training 
% using the Adam optimizer ~\cite{kingma2014adam} with a learning rate of $1\times10^{-1}$ and without any weight decay. 
% %without requiring any GPU
% For a sequence of 2000 frames, we found our optimization to converge after 2K iterations in 2 hours on average with 16 Intel Core i7 CPU cores. 
% Since our
% %reconstruction is a purely 
% skeleton model has only few parameters we run Step 1 and Step 2 on the CPU.

% In Step 3, we use the estimated pose and the bone rotations to learn $G(\theta)$. For occlusion handling, we use 20\% threshold for automatic overlap area detection. Similar to ~\cite{su2021nerf}, we sample a batch of 3072 rays in each iteration, and attribute 30\% of these rays to occlusion areas if occlusion is detected. We train the volumetric model for 200K iterations and jointly refine the 3D pose. As in ~\cite{su2021nerf}, we finetune the remaining body details for 145K, keeping pose fixed. As \cite{su2022danbo} does not refine pose, we train for a maximum of 300K iterations to learn the body model with the pose fixed. Optionally, \danred{we refine the 3D pose estimates from Step 2 with~\cite{su2021nerf} to provide better initialization for~\cite{su2022danbo}}. The training is done on 4 Nvidia-Tesla V100 GPU and takes a 4-6 days. For example, for a sequence of 1620 training frames trained with occlusion handling, \emph{Mirror DANBO w/ Occlusion} takes 30 hours for 300K iterations and \emph{Mirror A-NeRF w/ Occlusion}, including pose refinement and finetuning, takes 130 hours for up to 400K iterations. 

% \section{Camera Calibration Details}

% \paragraph{Hyperparameter selection.} Hyperparameters, including the number of RANSAC steps and the angle threshold for up-right poses used in the camera calibration are determined on camera 2 and 3 of the \emph{MirrorHuman-eval} set (our validation set). %\dan{Daniel: Add rebuttal response table for how degree threshold was selected?}

% \paragraph{Derivation.} Our single view calibration is based on \cite{tang2023anon}. For completeness, we provide an overview of the relevant steps below. The single view calibration method is based on the well-established direct linear transform (DLT)~\cite{sutherland1974three} method to solve projective relations. We first write our constraints as a linear system of equations that is solved using Singular Value Decomposition (SVD), up to the unknown scale factor arising from the projection. To reach the form $\mM \vx = 0$, we take the cross product on both sides of Eq.~1
% %\ref{eq:projection}
% and Eq.~2 from the main paper
% %\ref{eq:head}
% and subtract the \da{two} results to derive
% \begin{equation}
% \vq_\text{neck} \times K (\vp_\text{ankle} + \vn \cdot h) - \vq_\text{ankle} \times K (\vp_\text{ankle}) = 0,
% \label{eq:cross_prod}
% \end{equation}
% with $h$ the person height, $\vn$ the normal direction, and $\vq_\text{neck}$ and $\vq_\text{ankle}$ the neck and ankle positions. In the following we subscript variables with an $x,y,z$ to indicate the x,y,z-coordinates and with a number $1,2,3$ to refer to different person locations.
% %\begin{equation}
% %(\bar{x}_{ankle} \times C_{intrinsic}
% %\textbf{X}_{ankle}
% %\label{x_ankle_cross})
% %-
% %(\bar{x}_{head} \times C_{intrinsic}
% %(\textbf{X}_{head} + N\cdot h))
% %=
% %0
% %\label{cross_subtract}
% %\end{equation}



% In matrix form, using $\Delta\vq_x = \vq_x^\text{neck} - \vq_x^\text{ankle}$, $\Delta\vq_y = \vq_y^\text{neck} - \vq_y^\text{ankle}$, and $z$ to represent the unknown depth of the ankle, Eq.~\ref{eq:cross_prod} can be expressed as

% \begin{equation}
% \begin{pmatrix}
% 0 & -1 & \vq_y^\text{neck} & 0 & -1 & \Delta\vq_y \\ 1 & 0 & -\vq_x^\text{neck} & 1 & 0 & -\Delta\vq_x \\
% \end{pmatrix}
% \begin{pmatrix}
% f\vn_x \\ f\vn_y \\ \vn_z \\ \vn_z\vo_x \\ \vn_z\vo_y \\ z/h
% \end{pmatrix}
% = 0,
% \label{cross_matrix}
% \end{equation}
% where $f$ is the focal length and $\vo$ the principal point of the camera intrinsics $\mK$.
%  By using at least three 2D neck $\vq_\text{neck}$ and ankle $\vq_\text{ankle}$ detections, we form the constraint matrix
% \begin{equation}
% \textbf{D} =
% \begin{pmatrix}
% 0 & -1 & \vq_{y1}^\text{neck} & \Delta\vq_{y1} & 0 & 0\\ 1 & 0 & -\vq_{x1}^\text{neck} & -\Delta\vq_{x1} & 0 & 0\\
% 0 & -1 & \vq_{y2}^\text{neck} & 0 & \Delta\vq_{y2} & 0\\ 1 & 0 & -\vq_{x2}^\text{neck} & 0 & -\Delta\vq_{x2} & 0\\
% 0 & -1 & \vq_{y3}^\text{neck} & 0 & 0 & \Delta\vq_{y3}\\ 1 & 0 & -\vq_{x3}^\text{neck} & 0 & 0 & -\Delta\vq_{x3}
% \end{pmatrix}
% \label{eq: full_matrix}
% \end{equation}
% that gives the system of equations
% \begin{equation}
% \textbf{D} %\cdot
% \begin{pmatrix}
% f\vn_x + \vn_z\vo_x\\ f\vn_y + \vn_z\vo_y\\ \vn_z \\ z_1/h \\z_2/h \\ z_3/h
% \label{eq: DLT}
% \end{pmatrix}
% = 0
% .
% \end{equation}

% We solve Eq.~\ref{eq: DLT} using SVD. Having more than three ankles and necks results in an over-determined system, for which we can find a least-squares solution.

% \paragraph{Ground normal extraction.}

% Since Eq.~\ref{eq: DLT} is a $6 \times 6$ system with rank five, any solution we find is unique up to a scalar. In order to determine $\vn$ from the SVD or least-squares solution, we use the fact that the normal vector is perpendicular to any vector formed by a pair of ankles. Using

% \begin{equation}
%     \begin{bmatrix}
%     \bar{\vn_x}\\\bar{\vn_y}\\\bar{\vn_z}\\\bar{z_1}\\\bar{z_2}\\\bar{z_3}
%     \end{bmatrix}
%     = \lambda
%     \begin{bmatrix}
%     \vn_x + \vn_z\vo_x/f\\\vn_y + \vn_z\vo_y/f\\\vn_z/f\\z_1/(hf)\\z_2/(hf)\\z_3/(hf)
%     \end{bmatrix},
%     \label{svd_soln_apndx}
% \end{equation}
% %
% If we do not have a given focal length, we can derive the equation for the focal length,
% %
% \begin{equation}
% f = \sqrt{\frac{(-(\bar{\vn}_x - \bar{\vn}_z\vo_x)\bar{\vq}_\text{x} - 
% (\bar{\vn}_y - \bar{n}_z\vo_y)\bar{\vq}_\text{y})}{(\bar{\vn}_z(\bar{z}_1 - \bar{z}_2))}},
% \end{equation}
% %
% with 
% %
% \begin{equation}
% \bar{\vq}_\text{x} = ((\vq_{x1}^\text{ankle} - \vo_x)\bar{z}_1 - (\vq_{x2}^\text{ankle} - \vo_x)\bar{z}_2)
% p\end{equation}
% %
% and
% %
% \begin{equation}
% \bar{\vq}_\text{y} = ((\vq_{y1}^\text{ankle} - \vo_y)\bar{z}_1 - (\vq_{y2}^\text{ankle} - \vo_y)\bar{z}_2).
% \end{equation}


% Either the estimated \danred{focal lengths} or a given focal length enables us to recover $\lambda\vn$ and $\lambda$($z_1$, $z_2$, $z_3$). To
% remove $\lambda$, we divide both vectors by the $L_2$ norm of $\lambda\vn$, giving us a unique $\vn$ of length one and ankle depths $z_1$, $z_2$, and $z_3$.

% Using the normal vector $\vn$ and the known depths $z_1$, $z_2$, and $z_3$, we recover the orientation and position of the ground plane and subsequently estimate the mirror plane from a 3D ankle position of a person and its mirror image, as explained in the main document.

% {
%     \small
%     \bibliographystyle{ieeenat_fullname}
%     \bibliography{main}
% }


% \end{document}
